# Supplementary material for: LigBench: A Unified and Human-Aligned Benchmark for LLM-based Research Idea Generation
Source: arXiv:2608.13136 source file (2026-08-13)
Supplement: Supplementary file 3 [file Hyper-parameters_for_Fine-Tuning.tex]

\section{Hyper-parameters for Fine-Tuning}
\label{app:training_hyperparameter}

\begin{table}[htbp]
\centering
\caption{Hyper-parameters for Fine-Tuning.}
\begin{tabular}{l c}
    \toprule
    \textbf{Hyper-Parameter} & \textbf{Default Value} \\
    \midrule
    Finetuning Type & LoRA \\
    LoRA Target & all \\
    LoRA Rank & \num{16} \\
    LoRA Alpha & \num{16} \\
    LoRA Dropout & \num{0.05} \\
    \midrule
    Cutoff Length & \num{4096} \\
    \midrule
    Gradient Accumulation Steps & \num{16} \\
    Learning Rate & \num{1e-4} \\
    Train Epochs & \num{1.0} \\
    Learning Rate Scheduler & Cosine \\
    Warmup Ratio & \num{0.1} \\
    \bottomrule
\end{tabular}
\end{table}
